# Supplementary material for: Symmetry in Multiple Self-Consistent-Field Solutions of Transition-Metal Complexes
Source: arXiv:1909.03915 source file (2019-12-11)
Supplement: Supplementary file 1 [file qchemlanguage.tex]

% !TeX root = symmultiplescf-suppinfo.tex

\definecolor{eclipseBlue}{RGB}{42,0.0,255}
\definecolor{eclipseGreen}{RGB}{63,127,95}
\definecolor{eclipsePurple}{RGB}{127,0,85}

\lstdefinelanguage{QChemInput}
{
	%% List of keywords
	alsoletter = {_\$},
	% Rem variables
	keywords = [1]{
		SCF_MINFIND_INITNORM,
		BASIS,
		EXCHANGE,
		CORRELATION,
		UNRESTRICTED,
		SCF_GUESS,
		SCF_CONVERGENCE,
		SCF_ALGORITHM,
		SCF_MAX_CYCLES,
		MOM_START,
		PRINT_ORBITALS,
		SCF_PRINT,
		MAX_SCF_CYCLES,
		SYMMETRY,
		THRESH,
		DIIS_SEPARATE_ERRVEC,
		SYM_IGNORE,
		SCF_SAVEMINIMA,
		SCF_READMINIMA,
		SCF_MINFIND_INITNORM,
		SCF_MINFIND_INCREASEFACTOR,
		SCF_MINFIND_WELLTHRESH,
		SCF_MINFIND_RANDOMMIXING,
		SCF_MINFIND_NRANDOMMIXES,
		SCF_MINFIND_MIXMETHOD,
		SCF_MINFIND_MIXENERGY,
		SCF_MINFIND_RESTARTSTEPS,		
	},
	keywords = [2]{
		\$molecule,
		\$rem,
		\$rem_frgm,
		\$occupied,
		\$end,
	},
	comment = [l]{!},
	% Style
	sensitive = false, % keywords are not case-sensitive
	caption = \lstname,
	backgroundcolor = \color{Cornsilk},
	frame = trbl,
	numberstyle = \tiny\ttfamily\noncopy, % style of the line numbers
	numbers = left,
	% Syntax highlighting
	keywordstyle = [1]{\color{eclipsePurple}},
	keywordstyle = [2]{\color{Navy}},
	commentstyle = \color{eclipseGreen}
}

\lstdefinestyle{custombash}{
	language = bash,
	frame = trbl,
	backgroundcolor = \color{Seashell},
%	breakatwhitespace = true,
	breaklines = true,
	prebreak = \mbox{\textcolor{red}{\textbackslash}},
	postbreak = \mbox{\textcolor{Green}{\noncopy{>}}},
}

\lstdefinelanguage{QChemOutput}
{
	%% List of keywords
	alsoletter = {},
	keywords = [1]{
	},
	% Style
	sensitive = false, % keywords are not case-sensitive
	caption = \lstname,
	backgroundcolor = \color{Cornsilk},
	frame = trbl,
	numberstyle = \tiny\ttfamily\noncopy, % style of the line numbers
	numbers = left,
	% Syntax highlighting
}
