# Supplementary material for: Symmetry in Multiple Self-Consistent-Field Solutions of Transition-Metal Complexes
Source: arXiv:1909.03915 source file (2019-12-11)
Supplement: Supplementary file 2 [file results-d1-supp.tex]

% !TeX root = symmultiplescf-suppinfo.tex

\section{\ce{[TiF6]^{3-}}: Detailed Results}

	\begin{table*}
		\centering
		\caption{Overlap matrices for degenerate, linearly independent UHF solutions in \ce{[TiF6]^{3-}}.}
		\label{tab:TiF63-ovlap}
		\footnotesize
		\begingroup
		
		\scalebox{1}{
		\begin{subtable}[t]{\textwidth}
			\centering
			\caption{$\mathrm{A}_{\frac{1}{2}}$ solutions in \ce{[TiF6]^{3-}}.}
			\begin{tabular}[t]{%
					r |%
					*{6}{S[table-format=2.4, table-alignment=right]}
				}
				\toprule
				& $\mathrm{A}_{\frac{1}{2},1}$ & $\mathrm{A}_{\frac{1}{2},2}$ & $\mathrm{A}_{\frac{1}{2},3}$ & $\mathrm{A}_{\frac{1}{2},4}$ & $\mathrm{A}_{\frac{1}{2},5}$ & $\mathrm{A}_{\frac{1}{2},6}$ \\
				\midrule
				$\mathrm{A}_{\frac{1}{2},1}$ &  1.0000 & -0.4991 &  0.4991 & -0.4991 & -0.4991 &  0.0000 \\
				$\mathrm{A}_{\frac{1}{2},2}$ & -0.4991 &  1.0000 &  0.0000 & -0.4991 &  0.4991 &  0.4991 \\
				$\mathrm{A}_{\frac{1}{2},3}$ &  0.4991 &  0.0000 &  1.0000 & -0.4991 &  0.0000 & -0.4991 \\
				$\mathrm{A}_{\frac{1}{2},4}$ & -0.4991 & -0.4991 & -0.4991 &  1.0000 &  0.0000 & -0.4991 \\
				$\mathrm{A}_{\frac{1}{2},5}$ & -0.4991 &  0.4991 &  0.4991 &  0.0000 & 1.0000 & -0.4991 \\
				$\mathrm{A}_{\frac{1}{2},6}$ &  0.0000 &  0.4991 & -0.4991 & -0.4991 & -0.4991 & 1.0000 \\
				\bottomrule
			\end{tabular}
		\end{subtable}
		}
	
		\vspace{1cm}
		\scalebox{1}{
		\begin{subtable}[t]{.48\textwidth}
			\centering
			\caption{$\mathrm{A}'_{\frac{1}{2}}$ solutions in \ce{[TiF6]^{3-}}.}
			\begin{tabular}[t]{%
					r |%
					*{3}{S[table-format=2.4, table-alignment=right]}
				}
				\toprule
				& $\mathrm{A}'_{\frac{1}{2},1}$ & $\mathrm{A}'_{\frac{1}{2},2}$ & $\mathrm{A}'_{\frac{1}{2},3}$ \\
				\midrule
				$\mathrm{A}'_{\frac{1}{2},1}$ &  1.0000 &  0.0000 &  0.0000 \\
				$\mathrm{A}'_{\frac{1}{2},2}$ &  0.0000 &  1.0000 &  0.0000 \\
				$\mathrm{A}'_{\frac{1}{2},3}$ &  0.0000 &  0.0000 &  1.0000 \\
				\bottomrule
			\end{tabular}
		\end{subtable}
		}
		\hfill
		\scalebox{1}{
		\begin{subtable}[t]{.48\textwidth}
			\centering
			\caption{$\mathrm{B}_{\frac{1}{2}}$ solutions in \ce{[TiF6]^{3-}}.}
			\begin{tabular}[t]{%
					r |%
					*{3}{S[table-format=2.4, table-alignment=right]}
				}
				\toprule
				& $\mathrm{B}_{\frac{1}{2},1}$ & $\mathrm{B}_{\frac{1}{2},2}$ & $\mathrm{B}_{\frac{1}{2},3}$ \\
				\midrule
				$\mathrm{B}_{\frac{1}{2},1}$ &  1.0000 &  0.4988 & -0.4988 \\
				$\mathrm{B}_{\frac{1}{2},2}$ &  0.4988 &  1.0000 &  0.4988 \\
				$\mathrm{B}_{\frac{1}{2},3}$ & -0.4988 &  0.4988 &  1.0000 \\
				\bottomrule
			\end{tabular}
		\end{subtable}
		}
		\endgroup
	\end{table*}

	\begin{table}
		\centering
		\caption{
			Energies and $\langle \hat{S}^2 \rangle$ values of $M_S = \frac{1}{2}$ UHF solutions in \ce{[TiF6]^{3-}}.
		}
		\label{tab:d1_uhfenergy}
		\footnotesize
		\begingroup
		
		\begin{tabular}[t]{%
			>{\raggedright\arraybackslash}m{0.9cm}%
			S[table-format=4.7, table-alignment=left]%
			S[table-format=1.4, table-alignment=left]%
		}
			\toprule
			$\Psi_\mathrm{UHF}$ &	{Energy/\si{\hartree}} & {$\langle \hat{S}^2 \rangle$} \\
			\midrule
			$\mathrm{A}_{\frac{1}{2}}$ & -1444.9306822 & 0.7522 \\
			$\mathrm{A}_{\frac{1}{2}}'$ & -1444.9306706 & 0.7522 \\
			$\mathrm{B}_{\frac{1}{2}}$ & -1444.8666826 & 0.7527 \\
			\bottomrule
		\end{tabular}
		\endgroup
	\end{table}

	\begin{table}
		\centering
		\caption{
			Energies and $\langle \hat{S}^2 \rangle$ values of $M_S = \frac{1}{2}$ NOCI wavefunctions in \ce{[TiF6]^{3-}}.
		}
		\label{tab:d1_nocienergy}
		\footnotesize
		\begingroup
		
		\begin{tabular}[t]{
				>{\raggedright\arraybackslash}m{2.7cm}%
				S[table-format=4.7, table-alignment=left]%
				S[table-format=1.4, table-alignment=left]}
			\toprule
			$\Phi$ &	{Energy/\si{\hartree}} & {$\langle \hat{S}^2 \rangle$} \\
			\midrule
			$\prescript{2}{}{T}_{2g}[\mathrm{A}_{\frac{1}{2}}]$ & -1444.9326372 & 0.7512 \\
			$\prescript{\varnothing}{}{T}_{1g}[\mathrm{A}_{\frac{1}{2}}]$ & -1442.6252833 & 1.8403 \\
			\midrule
			$\prescript{2}{}{T}_{2g}[\mathrm{A}_{\frac{1}{2}}\oplus\mathrm{A}_{\frac{1}{2}}']$ & -1444.9327765 & 0.7512 \\
			$\prescript{\varnothing}{}{T}_{2g}[\mathrm{A}_{\frac{1}{2}}\oplus \mathrm{A}_{\frac{1}{2}}']$ & -1442.6931022 & 1.5549 \\
			$\prescript{\varnothing}{}{T}_{1g}[\mathrm{A}_{\frac{1}{2}}\oplus \mathrm{A}_{\frac{1}{2}}']$ & -1442.6252833 & 1.8403 \\
			\midrule
			$\prescript{2}{}{E}_g[\mathrm{B}_{\frac{1}{2}}]$ & -1444.8682433 & 0.7517 \\
			$\prescript{\varnothing}{}{A}_{2g}[\mathrm{B}_{\frac{1}{2}}]$ & -1442.9308067 & 2.0321 \\
			\bottomrule
		\end{tabular}
		\endgroup
	\end{table}

	\clearpage
